# Supplementary material for: Finding Label and Model Errors in Perception Data With Learned Observation Assertions
Source: arXiv:2201.05797 source file (2022-01-15)
Supplement: Supplementary file 1 [file appendix.tex]

\appendix

\section{API}
\begin{lstlisting}
class Observation:
    pass

class ObservationBundle:
  def add_observation(self, obs: Observation)
      -> None
  def is_associated(self, obs: Observation)
      -> boolean
  # Is there a better name than
  # "is_associated"?

class ObservationPrior:
  def score(self, ob: Observation)
      -> float
  def project(self, ob: Observation)
      -> Sequence[float]

  def _fit(self, obs: Sequence[Observation])
      -> None
  def _serialize(self, location: str)
      -> None
    
class ObservationBundlePrior:
    ...

class TransitionPrior:
    ...
    
class Track:
  def add_bundle(self, ob: ObservationBundle)
      -> None
  def add_single_prior(self, sp: SinglePrior)
      -> None
  def add_trans_prior(self, tp: TransPrior)
      -> None
  def add_end_prior(self, ep: EndPrior)
      -> None
  def finalize(self) -> None

  def last_bundle(self) -> ObservationBundle
  def score(self) -> float
\end{lstlisting}
